# Supplementary material for: Instantaneous physics-based ground motion maps using reduced-order modeling
Source: arXiv:2212.11335 ancillary file (2023-07-26)
Supplement: Supplementary file 1 [file supplement.pdf]

# Supporting Information for "Instantaneous physics-based ground motion maps using reduced-order modeling"

John M. Rekoske[1], Alice-Agnes Gabriel[1,2], Dave A. May[1]

[1]Scripps Institution of Oceanography, University of California, San Diego

[2]Department of Earth and Environmental Sciences, Ludwig-Maximillians-Universität München, Munich, Germany

## Contents of this file

1. Tables S1 to S2
2. Figures S1 to S9
3. Movie S1

## Introduction.

This supporting information provides two additional tables that list the details of the layer over halfspace (LOH) velocity model (Table S1) and the selected hyperparameters for our ROMs using different types of function approximators (Table S2). We also provide figures for our analysis of the distances between the parameters in the testing and training datasets (Figure S1). We plot the testing dataset errors against the distances in Figure S2, and compare these errors with a simple approach of using the nearest-neighbor PGV map (Figure S3). Also shown are the complete histograms of the errors on the testing dataset (Figures S4 and S5), the errors for the particular site of interest used in the

paper (Figure S6), the correlation between mean absolute percentage errors and source parameters (Figure S7), our analysis of the PGV inter-event terms (Figure S8), and the FOM PGV values at the site of interest (Figure S9). Lastly, we provide a movie that dynamically shows how the peak-ground velocity maps are constructed from the basis vectors (Movie S1).

**Table S1.** Parameter values for the layer over halfspace (LOH) velocity model.

| Parameter | Value |
|---|---|
| Thickness of layer | 2.0 km |
| $V_S$ of layer | 2.0 km/s |
| $V_P$ of layer | 4.0 km/s |
| $\rho$ of layer | 2600 kg/m$^3$ |
| $V_S$ of halfspace | 3.464 km/s |
| $V_P$ of halfspace | 6.0 km/s |
| $\rho$ of halfspace | 2700 kg/m$^3$ |

**Table S2.** Hyperparameters selected by cross-validation for each type of function approximator.

| Approximator | Hyperparameter | Value |
|---|---|---|
| RBF | kernel | quintic |
| MLP | hidden layers | (200, 200) |
| MLP | no. of outputs | 30 |
| kNN | k | 5 |
| RF | number of trees | 50 |

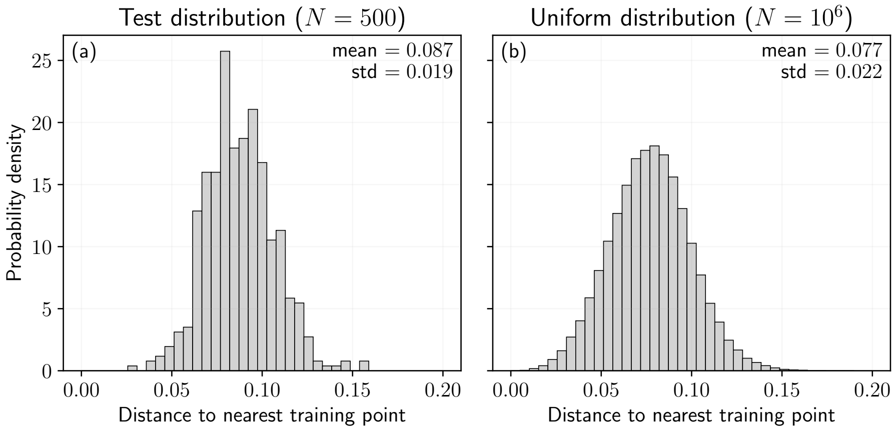


**Figure S1.** (a) probability distribution of the Euclidean distances from each parameter in $\boldsymbol{P}_{\text{test}}$ to the nearest parameter in $\boldsymbol{P}_{\text{train}}$. (b) same as panel (a), but for $\boldsymbol{P}_{\text{uniform}}$ instead of $\boldsymbol{P}_{\text{test}}$.

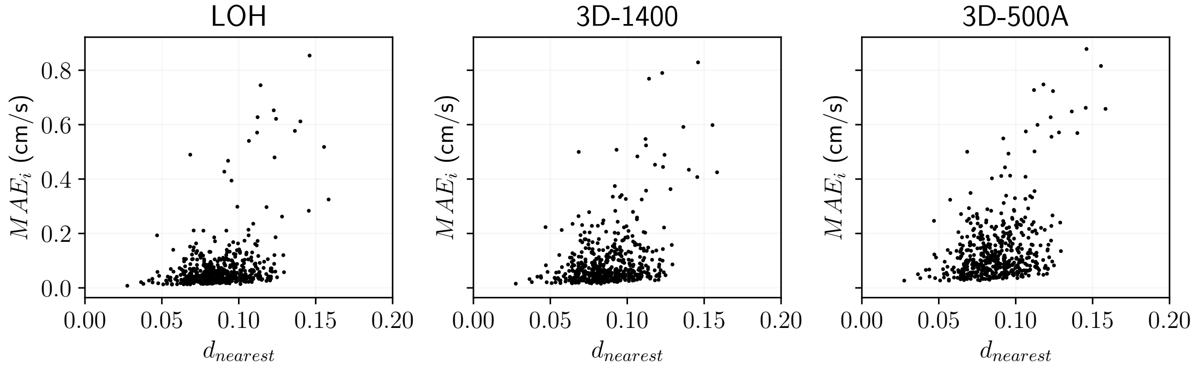


**Figure S2.** Testing dataset errors for the LOH (left) 3D-1400 (middle), and 3D-500A forward models (right), plotted as a function of the Euclidean distance to the nearest training parameter ($d_{\text{nearest}}$).

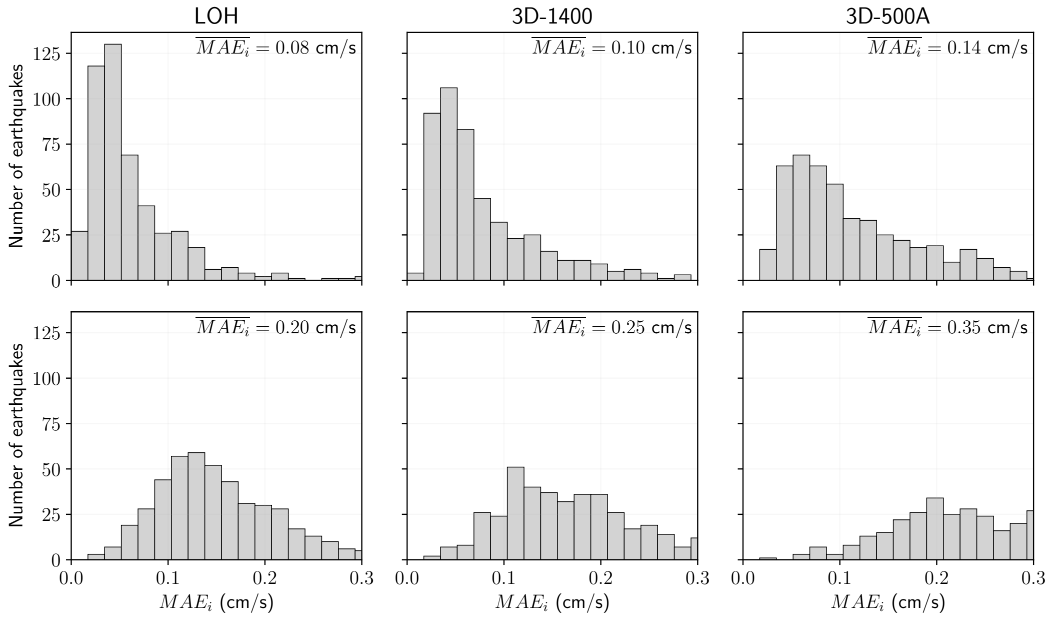


**Figure S3.** Comparison of the ROM errors (top row) and the errors resulting from selecting the nearest PGV map (bottom row). Errors are shown for the LOH (left), 3D-1400 (middle), and 3D-500A forward models (right column).

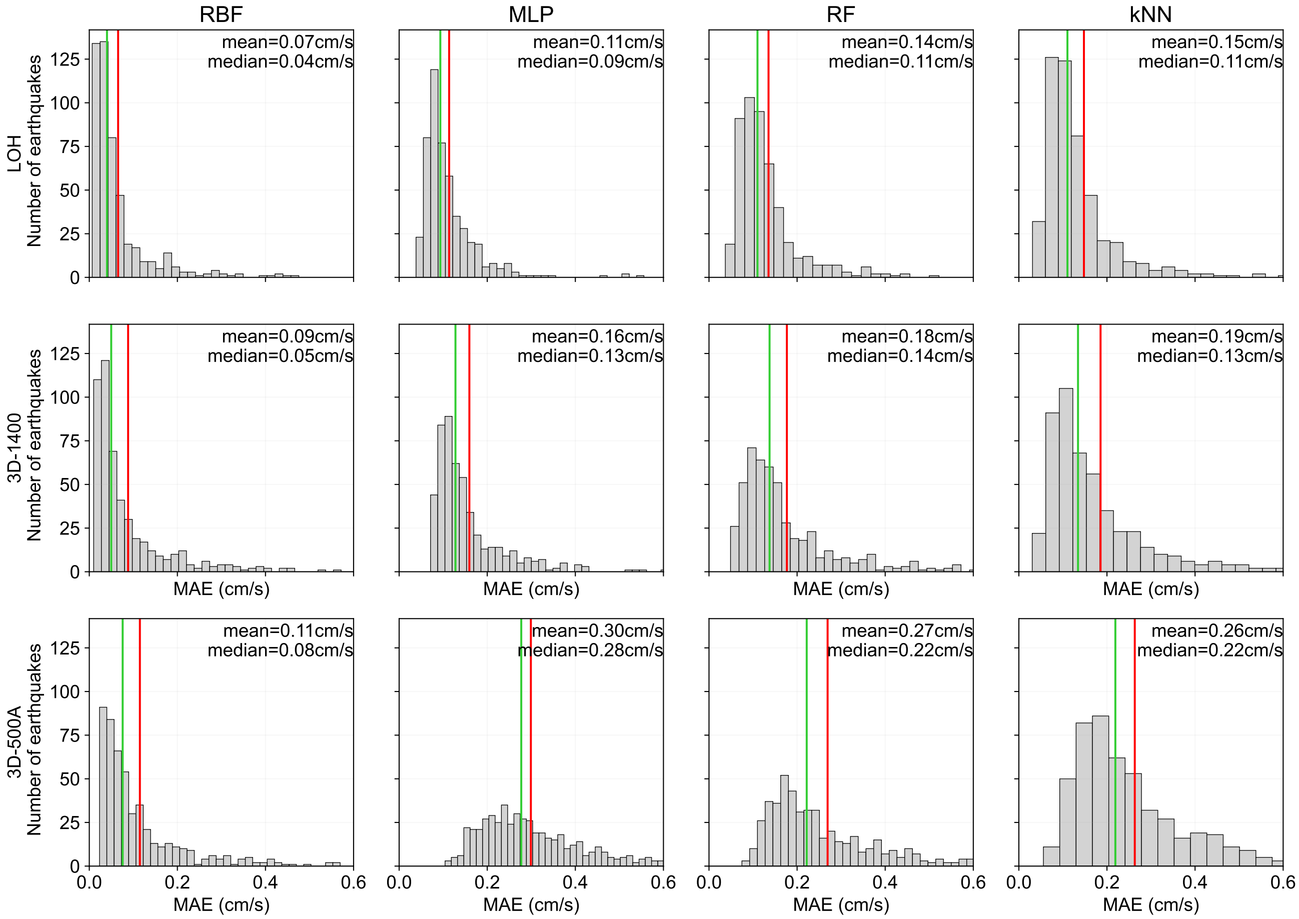


**Figure S4.** Histograms of the mean absolute errors (MAE) on the testing dataset. Each row shows the errors for a different forward model (LOH, top; 3D-1400, middle; 3D-500A, bottom). Each column is for a different function approximator used in iPOD. The mean of each distribution is indicated with a solid red line, and the median with a solid green line. The values of the mean and median are indicated in the upper right corner of each panel.

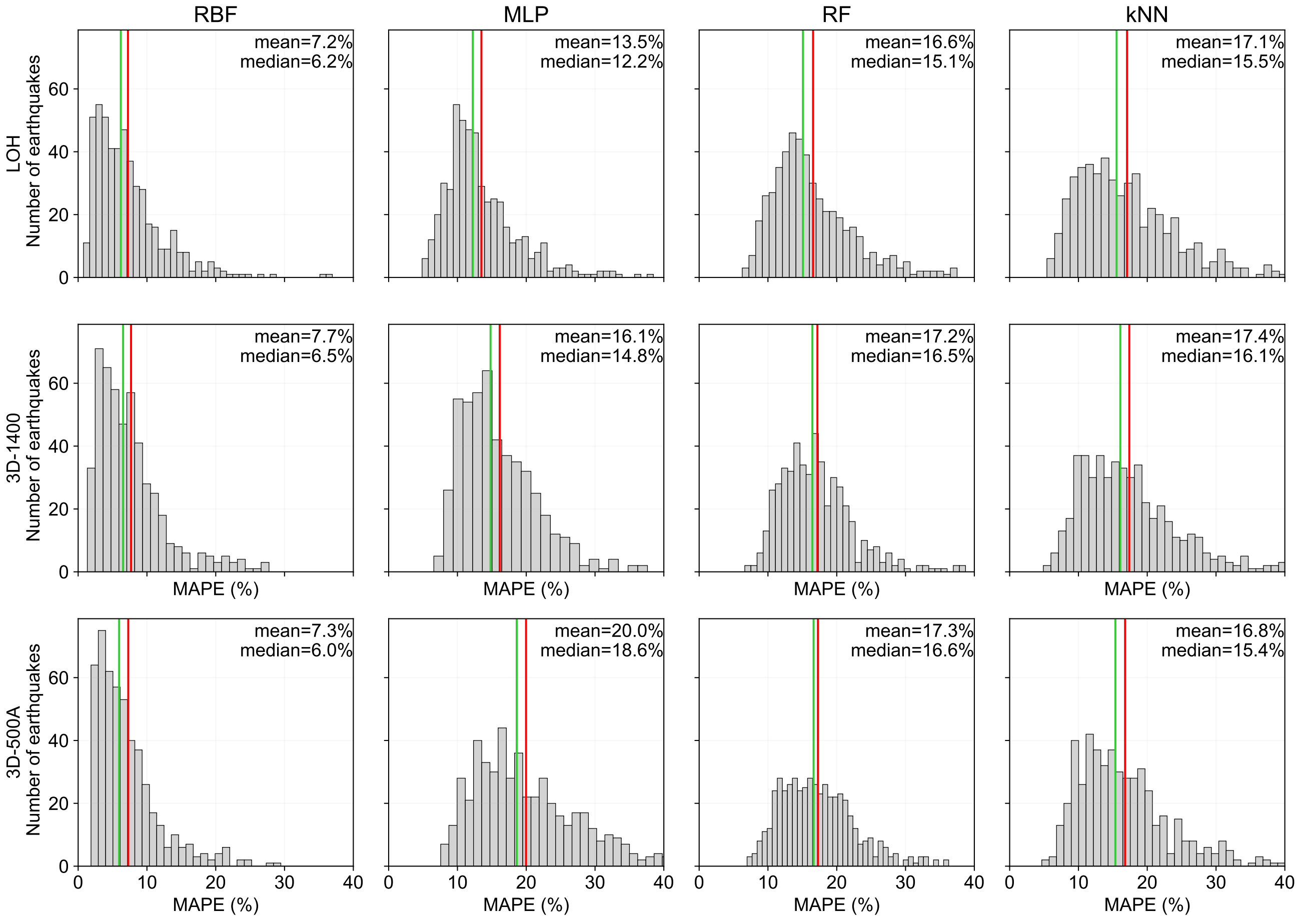


**Figure S5.** Same as Figure S4, but showing the mean absolute percentage error (MAPE) histograms instead of MAE.

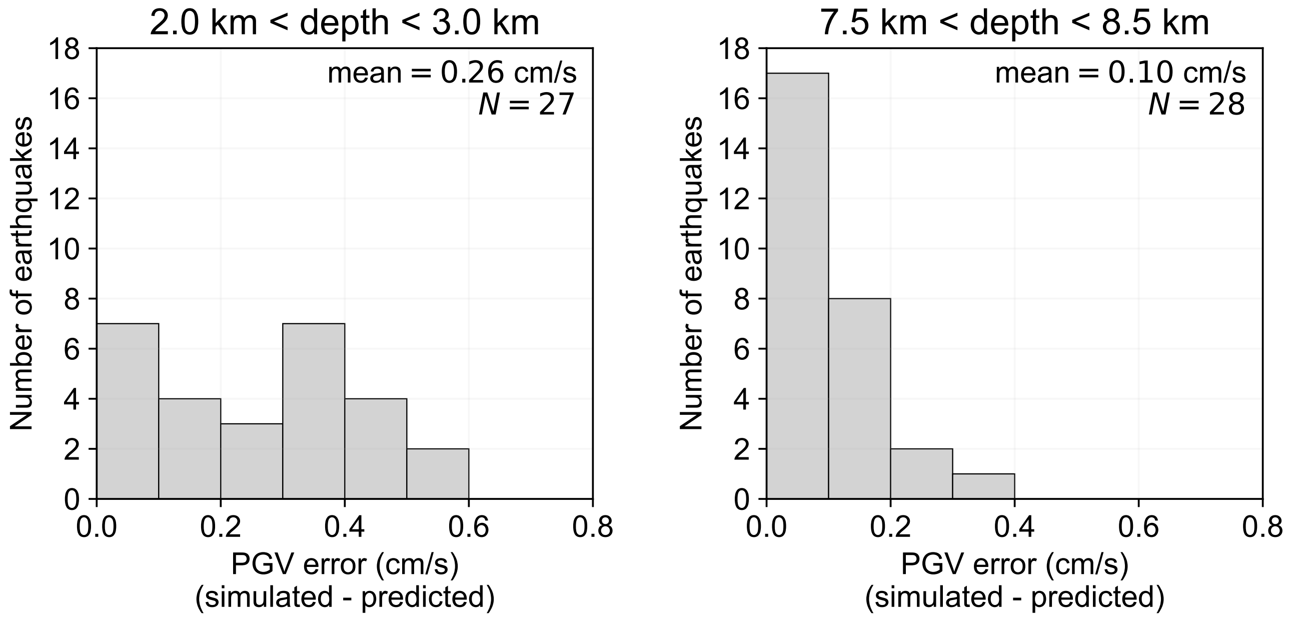


**Figure S6.** PGV errors on the testing dataset for the chosen site of interest located near the Clearwater Power Plant. The left panel shows the errors for shallow sources with hypocentral depths between 2.0 and 3.0 km. The right panel shows errors for deeper sources with hypocentral depths between 7.5 and 8.5 km. The mean absolute error ($MAE$) and total number of earthquakes ($N$) for each panel are indicated in the upper right corners.

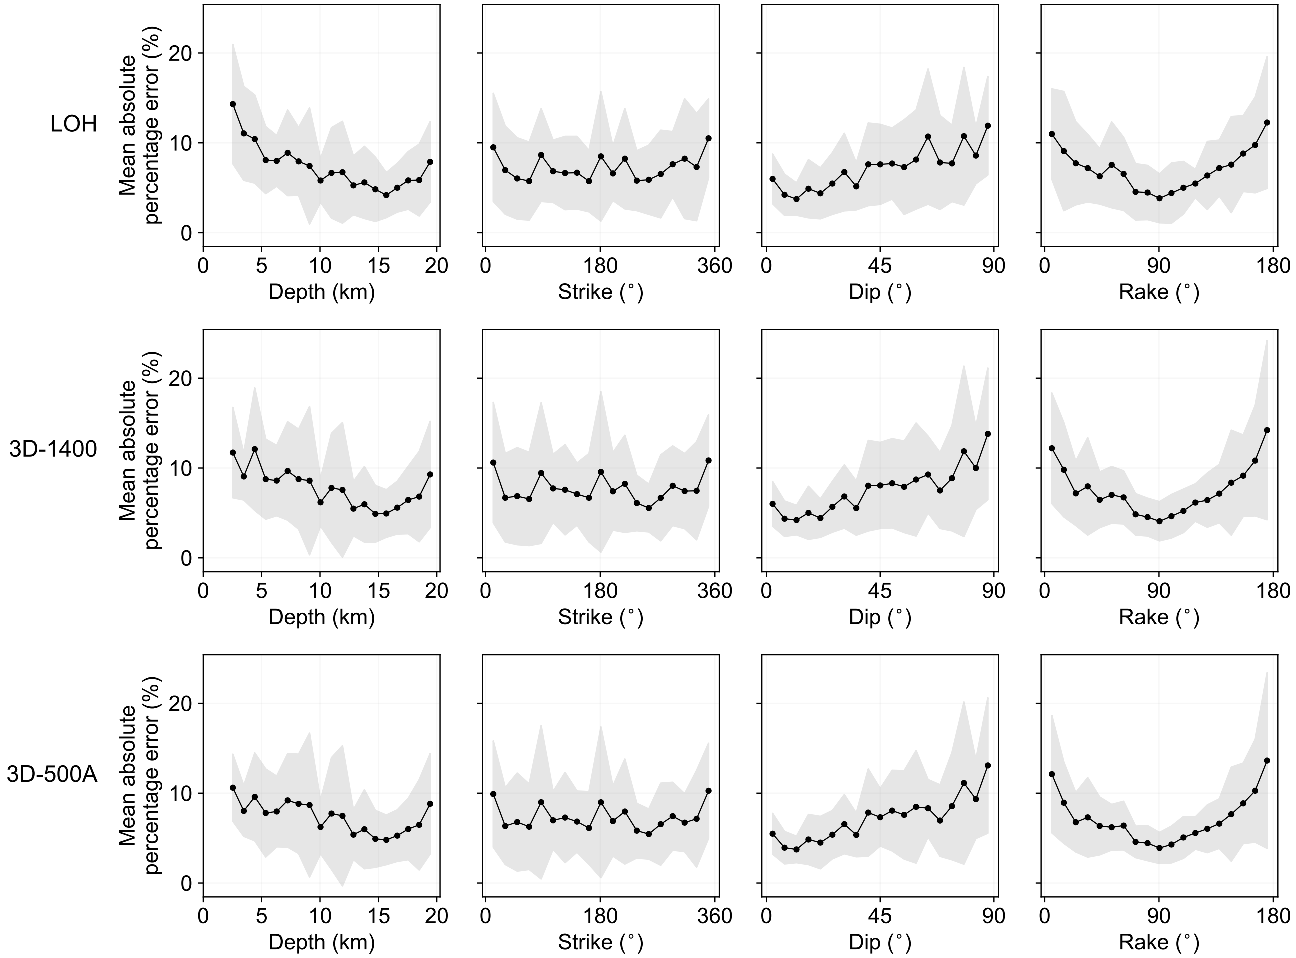


**Figure S7.** Mean absolute percentage errors plotted against the source parameters for the LOH (top), 3D-1400 (middle), and 3D-500A (bottom) forward problems.

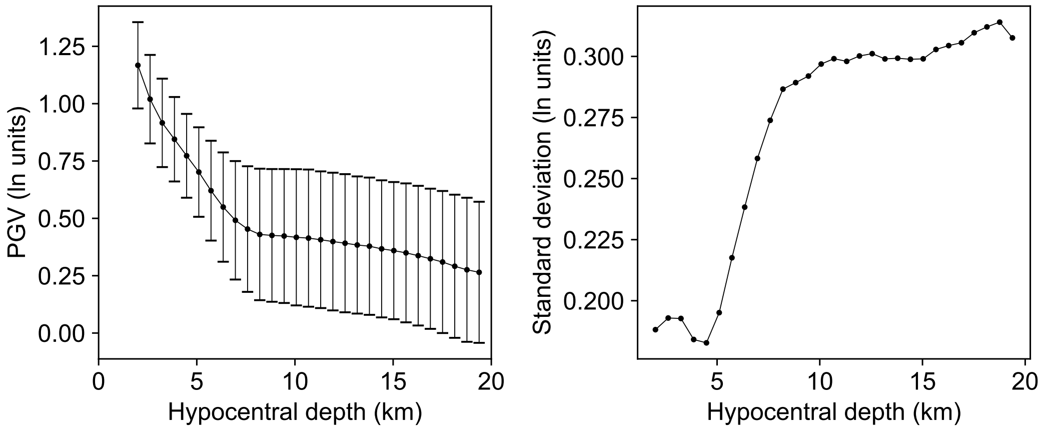


**Figure S8.** ROM PGV predictions at the site of interest for varying source depths and focal mechanisms, plotted against the hypocentral depth (left). The error bars indicate plus or minus one standard deviation in each of the 30 depth bins. Standard deviations plotted against the hypocentral depth (right).

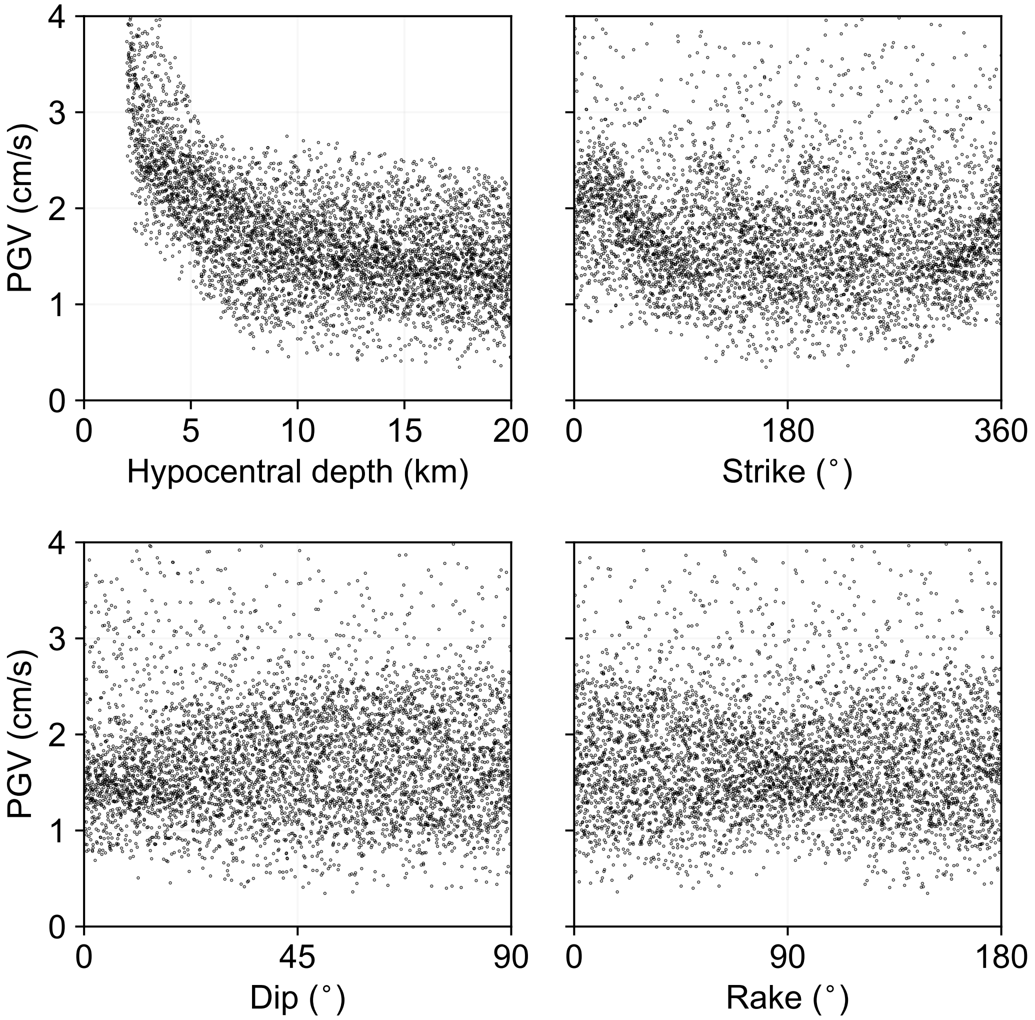


**Figure S9.** FOM PGV measurements at the site of interest for the complete set of 5000 FOM simulations.
